# Supplementary material for: CapsNet for Medical Image Segmentation
Source: arXiv:2203.08948 source file (2022-03-16)
Supplement: Supplementary file 1 [file appendix01.tex]

\begin{frontmatter}
\chapter{Appendix title}%\label{chap:appa}
\end{frontmatter}

%\section{}\label{}
