# Supplementary material for: CapsNet for Medical Image Segmentation
Source: arXiv:2203.08948 source file (2022-03-16)
Supplement: Supplementary file 2 [file appendix02.tex]

\begin{frontmatter}
\chapter{Appendix title}%\label{chap:appb}
\end{frontmatter}
